# Supplementary material for: Towards Seamless Tracking-Free Web: Improved Detection of Trackers via One-class Learning
Source: arXiv:1603.06289 source file (2016-03-20)
Supplement: Supplementary file 1 [file appendixb.tex]

\begin{table*}[t]
\centering
%\begin{tabular}{lll}
\caption{Ghostery replaces tracking JavaScript programs (in the right-most column) with Surrogate JavaScript programs (second column). Ghostery (version \# 5.4.1) has surrogate JavaScript programs for only 50 trackers.}
\begin{tabularx}{\linewidth}{  r X X }
\toprule
\toprule
ID	 & Surrogate JavaScript programs (Replacement)	& Linked To (Sources)\\
\hline
1 & \verb|var urchinTracker=function(){} ...| & \verb|www.google-analytics.com/ga.js|\\
2 & \verb|var _ga_ = document.querySelectorAll ...| & \verb|www.google-analytics.com/ga.js|\\
3 & \verb|var COMSCORE={beacon:function(){},purge: function(){ }}...| & \verb|b.scorecardresearch.com/beacon.js|\\
4 & \verb|var SavePageView= function(){ }, ...| & \verb|2912a.v.fwmrm.net/*| \\
5 & \verb|var YWA={getTracker:function(){}}... | & \verb|y.analytics.yahoo.com/fpc.pl|\\
6 &  \verb|function omn_rmaction() {...}| & \verb|www.aexp-static.com/api/axpi/ omniture/s_code.js|\\
7 & \verb|function geoip_country_code(){return 'A1';}; ...| & \verb|www.dwin1.com/4102.js| \\
8 & \verb|var geoip_city=geoip_region=geoip_region_name| & \verb|j.maxmind.com/app/geoip.js| \\
9 & \verb|function _ghost(){return{record : function(){ }}}...| & \verb|secure-au.imrworldwide.com/v60.js|\\
10 & \verb|function wt_sendinfo(){...};| & \verb|js.welt.de/resources/js/544/webtrekk.js| \\
11 & \verb|function mktoMunchkinFunction(){}; ... | & \verb|munchkin.marketo.net/munchkin.js|\\
12 & \verb|var stLight={subscribe:function(){}, options: function(){}}; ...| & \verb|w.sharethis.com/button/buttons.js|\\
13 & \verb|var addthis={init:function(){}, layers:function(){}, ...}|  & \verb|s7.addthis.com/js/300/addthis_widget.js| \\
14 & \verb|var DM_addEncToLoc= function(){},DM_tag= function(){...};| & \verb|js.revsci.net/gateway/gw.js|\\
15 & \verb|var SmartAdServer=SmartAdServerAjax  ...|  & \verb|cdn1.smartadserver.com/ diff/251/smartad.js| \\
16 & \verb|var _cm= function(){}; _cm.prototype= function(){};... | & \verb|libs.coremetrics.com/v4.16.5/eluminate.js|\\
17 & \verb|var ATGSvcs= {l10n:{register :function(){}}, ...}| & \verb|static.atgsvcs.com/js/atgsvcs.js| \\
18 & \verb|var Ya=Ya or {};Ya.share= function(){var API={}; ...}|  & \verb|yandex\\.st\\/share\\/| \\
19 & \verb|function geoplugin_request(){ return   '0.0.0.0'; }; function ...| & \verb|www.geoplugin.net/extras/cookielaw.js|\\
20 & \verb|FB= {api:function(){ }, ...}| & \verb|connect.facebook.net/en_US/all.js|\\
21 & \verb|var fb = document.querySelectorAll(...)| & \verb|news.yahoo.com| \\
22 & \verb|function dcsMultiTrack(){};function ... | & \verb|*/js/webtrends/LIVE/WTID.js| \\
23 & \verb|function _hbRedirect(a,b,c){ location.href=c }; ...| & \verb|\\/hbx(.*)?\\.js| \\
24 & \verb|function mboxCreate(){ }; function mboxTrack(){return true; };...| & \verb|\\/(mbox)(.*)?\\.js| \\
25 & \verb|var s= {_noSuchMethod_:function(){ }, ...}| & \verb|o.aolcdn.com/os/omniture/prod/omniunih_portal_min.js|\\
26 & \verb|var s= {_noSuchMethod_: function(){}...}| & \verb|download.premiereradio.net/ track/s_code.js|  \\
27 & \verb|function linkCode(){csmonitor.com }; var s_time=...| & \verb|*/(omniture or omniunih).js| \\
28 & \verb|AC.Tracking.pageName= function(){};| & \verb|AC.Tracking.pageName='us'|\\
29 & \verb|var gapi={plusone:{ render:function(){},go: function(){ ... }}};| & \verb|apis.google.com/js/plusone.js|\\
30 & \verb|var gigya={accounts:{addEventHandlers: function(){ } }...}| & \verb|cdn.gigya.com/JS/socialize.js| \\
31 & \verb|function quantserve(){...} | & \verb|edge.quantserve.com/quant.js| \\
32 & \verb|function st_go(){ }; function linkclick(event) {...}| & \verb|stats.wordpress.com/e-201451.js| \\
33 & \verb|var mpq={track: function(a,b,c)...}| & \verb|cdn.mxpnl.com/libs/mixpanel-2.2.min.js| \\
34 & \verb|var OAS_RICH= OA_show= function(){ ... }| & \verb|var OAS_RICH=OA_show('**')| \\
35 & \verb|var GA_googleFillSlot= GA_googleFetchAds ...| & \verb|pagead2.googlesyndication.com/pagead/show_ads.js| \\
36 & \verb|var LM = {init:function(){ },complete: function(func){ func();}}| & \verb|esp3.locayta.com/venda.js| \\
37 & \verb|Typekit={ };CN.stats={ omniture:...}| & \verb|\\/(omniture or omniunih)(.*)?\\.js| \\
38 & \verb|var googletag={ };googletag.cmd={ }; ...| & \verb|www.googletagservices.com/tag/js/gpt.js|\\
39 & \verb|var Typekit={load: function(){ }}; ... | & \verb|use.typekit.net/wth6gwt.js|\\
40 & \verb|var Gravatar={ my_hash:' ',profile_cb: function(){ }...}| & \verb|http://s.gravatar.com/js/gprofiles.js|\\
41 & \verb|var Sailthru={setup: function(){}}; | & \verb|ak.sail-horizon.com/horizon/v1.js|  \\
42 & \verb|var pi={Track:function(){}}; | & \verb|t.qservz.com/js/pi.js| \\
43 & \verb|var mm\_variables=' ', mm_rules={...}| & \verb|www.mongoosemetrics.com/jsfiles/js-correlation/mm-getvar.js|\\
44 & \verb|var xt_adc=xt_click=xt_med=xt_rm =function()...| & \verb|s.tf1.fr/mmdia/static/xt/xtcore.js|\\
45 & \verb|var BV={configure:function(){},ui:function(){}}| & \verb|exxonmobil.ugc.bazaarvoice.com/ static/4445-en_us/bvapi.js|\\
46 & \verb|var brightcove={createExperiences: function(){}}| & \verb|admin.brightcove.com/js/BrightcoveExperiences.js|\\
47 & \verb|function adSetAdURL(){};function adSetMOAT(){}; ...| & \verb|o.aolcdn.com/ads/adsWrapper.js|\\
48 & \verb|var utag={link:function(){}}| & \verb|tags.tiqcdn.com/utag/advancedigital/nj/prod/utag.js|\\
49 & \verb|optimizely={};optimizely.activeExperiments= [];| & \verb|cdn.optimizely.com/js/128727546.js|\\
50 & \verb|cxApi={setCookiePath:function(){}, chooseVariation: function(){}}| & \verb|www.google-analytics.com/ cx/api.js|\\
\bottomrule
\bottomrule
%\end{tabular}
\end{tabularx}
%  \caption{Ghostery's Surrogate For Trackers}
  \label{tab:GhSurrogate}
\end{table*}

\newpage

\begin{table*}[t]
\centering
%\begin{tabular}{lll}
  \caption{NoScript replaces tracking JavaScript programs (in the right-most column) with Surrogate JavaScript programs (second columns). NoScript (version \# 2.6.9.11) has surrogate JavaScript programs for only 42 trackers.}
\begin{tabularx}{\linewidth}{  r X X }
\toprule
\toprule
%\multicolumn{2}{c}{Item} \\
%\cmidrule(r){1-2}
ID	 & Surrogate Scripts (Replacement)	& Linked To (Sources)\\
\hline
1 & \verb| Object.defineProperty (window,'adblock',{get:function() ...} | & \verb| @www.360haven.com|\\
2 & \verb|var _ga_ = document.querySelectorAll ...| & \verb|js.adscale.de|\\
3 & \verb|var COMSCORE={beacon: function(){},purge: function(){ }}...| & \verb|pagead2.googlesyndication.com|\\
4 & \verb|var SavePageView=function(){ },GetQueryStringValue ...| & \verb|^http://ads\.adtiger\.|\\
5 & \verb|var YWA={getTracker: function(){}}| & \verb|^http://bdv\.bidvert|\\
6 & \verb|function omn_rmaction() {}| & \verb|^http://view\.binlay(?:er)\.|\\
7 & \verb|function geoip_country _code(){return 'A1';};| & \verb|^http://intext\.mirago\.| \\
8 & \verb|var geoip_city=geoip_region=geoip_region_name| & \verb|^http://get\.mirando\.| \\
9 & \verb|function _ghost(){return{record:function(){}}}...| & \verb|.adagionet.com|\\
10 & \verb|function $wt_sendinfo(){}|; & \verb|s7.addthis.com/*addthis_widget.js| \\
11 & \verb|function mktoMunchkinFunction(){}; ... | & \verb|!@^https?://adf.ly/\w+/?$|\\
12 & \verb|var stLight={subscribe: function(){},options :function(){}; ...}| & \verb|ad.adriver.ru/ cgi-bin/erle.cgi|\\
13 & \verb|var addthis={init:function(){}, layers:function(){}, ...};|  & \verb|!https://addons.mozilla.org/| \\
14 & \verb|var DM_addEncToLoc=function(){},DM_tag= function(){}; | & \verb|!@digg.com/newsbar/*|\\
15 & \verb|var SmartAdServer=SmartAdServerAjax  ...$|  & \verb|!@^http://(?:dimtus or imageteam)\.(?:com, org)/img-| \\
16 & \verb|var _cm=function(){}; _cm.prototype= function(){};... | & \verb|>.disqus.com/*/build/themes/t_c4...b.js*|\\
17 & \verb|var ATGSvcs={l10n:{register: function(){}}, ...};| & \verb|connect.facebook.net| \\
18 & \verb|var Ya=Ya or {};Ya.share= function(){var API={}; ...}|  & \verb|*.google-analytics.com| \\
19 & \verb|function geoplugin_request() {return '0.0.0.0' ;}; function ...| & \verb|!@^https?://[^/]+google\..*/search|\\
20 & \verb|FB={api:function(){}, ...}| & \verb|!^https?://www\.google\.[a-z]+/search| \\
21 & \verb|googletag={__noSuchMethod__:function()this,...}| & \verb|.googletagservices.com|\\
22 & \verb|with(Gravatar={my_hash:' '})profile_cb=init= function(){};| & \verb|.gravatar.com|\\
23 & \verb|(function(){...})| & \verb|!@*.imagebam.com|\\
24 & \verb|document.body.insertBefore(...)| & \verb|!http://imagebunk.com/image/*|\\
25 & \verb|['agreeCont','TransparentBlack']...| & \verb|!@*.imagehaven.net|\\
26 & \verb|addEventListener('DOMContentLoaded',...)| & \verb|@*.imdb.com/video/*|\\
27 & \verb|let b=document.querySelector ( 'input[value= "YES"]')...| & \verb|!imgreserve.com|\\
28 & \verb|__defineSetter__('interstitialBox',...)| & \verb|@*.imagevenue.com|\\
29 & \verb|Invodo={__noSuchMethod__:function(){}}| & \verb|.invodo.com|\\
30 & \verb|let s=document.querySelector(...);if(s)s...)| & \verb|!@^https?:|\\
31 & \verb|document.cookie='noscript=; domain=.facebook.com;| & \verb|@*.facebook.com|\\
32 & \verb|if(typeof navigator.id==='undefined'){...}| & \verb|login.persona.org|\\
33 & \verb|for each(let s in document. getElementsByTagName ( 'script' )) {...}|  & \verb|!*.picbucks.com|\\
34 & \verb|location.replace(location.href.replace (...));| & \verb|!^https?://picsee\.net/2\d.*\.html|\\
35 & \verb|gapi=(function(){var f=arguments.callee;...}| & \verb|apis.google.com/js/plusone.js|\\
36 & \verb|(function(){var unloading=false; addEventListener (...)}| & \verb|"@^http:\/\/[\w\-\.]+\.[a-z]+ wyciwyg:"|\\
37 & \verb|window.quantserve=function(){}| & \verb|*.quantserve.com|\\
38 & \verb|rsinetsegs=[];DM_addEncToLoc=DM_tag= function(){};| & \verb|js.revsci.net|\\
39 & \verb|window.skimlinks=function(){}| & \verb|.skimlinks.com/api/|\\
40 & \verb|twttr=(function(){var f=arguments.callee;...}| & \verb|platform.twitter.com|\\
41 & \verb|for each(let l in document.links)if(/^https: ...| & \verb|!@.uniblue.com .liutilities.com|\\
42 & \verb|rmAddKey=rmAddCustomKey=rmShowAd ...| & \verb|*.yieldmanager.com|\\
\bottomrule
\bottomrule
\end{tabularx}
  \label{tab:NsSurrogate}
\end{table*}
