# Supplementary material for: Towards Seamless Tracking-Free Web: Improved Detection of Trackers via One-class Learning
Source: arXiv:1603.06289 source file (2016-03-20)
Supplement: Supplementary file 2 [file appendixc.tex]

Table \ref{tab:GTable} contains Rules for finding finding the ground truth. 
\begin{table*}[H]
\centering
%\begin{tabular}{lll}
\begin{tabularx}{\linewidth}{ c c c X  }
\toprule
%\multicolumn{2}{c}{Item} \\
%\cmidrule(r){1-2}
%\bottomrule
%\toprule
Rule	 & Useful/Useless & No. of Elements & Description\\
%\midrule
\toprule
R1 & Useless & 265 & All ads related JavaScripts (JS)\\
R2 & Useless & 157 & All social plugins, sdks, and widgets' JS\\
R3 & Useless & 156 & All cookies reader/writer JS\\
R4 & Useless & 147 & All third party service providers except CDNs (either first or third party)\\
R5 & Useless & 454 & All embedded JS that calls or use external JS\\
R6 & Useless & 493 & All web analaytics, dynamic ads, tracking, helper function, and market research\\
R7 & Useless & 54 & All cookies enabler\\
R8 & Useful & 542 & All linked JS (in page or linked) that provide function navigation, search, user interaction, etc\\
R9 & Useful & 609 & All embedded JS that provide functions like navigation, search, user interaction, etc\\
R10 & Useful & 132 & All CDNs (first party or third party)\\
R11 & Useless & 3 & All invisible, ads, or tracking iframes\\
R12 & Useless & 40 & All Javascripts in invisible iframes that writes and reads from/to cookies and local storage\\
R13 & Useful & 45 & All Javascript for event tracking like mouse or caps on/off\\
%\bottomrule
\toprule
\end{tabularx}
  \caption{Rules for Ground Truth Data}
  \label{tab:GTable}
\end{table*}
